# Supplementary material for: Semantic Residual Vector Quantization for Sign Language Generation
Source: arXiv:2611.06781 source file (2026-11-08)
Supplement: Supplementary file 1 [file supp_length_sensitivity.tex]

\subsection{Length Sensitivity of DTW}
\label{sec:supp_length_sensitivity}

We further test whether SOKE-style DTW scores are sensitive to prediction length.
Starting from the same generated Phoenix-2014T motions, we truncate the generated sequence by evaluating only the first fraction of predicted frames.
This is a diagnostic length-truncation experiment rather than a generation method.
\cref{tab:supp_length_sensitivity} shows that shortening the evaluated prediction improves DTW-based distances while substantially degrading retrieval and FID.
For example, reducing the effective length from 100\% to 50\% improves left-hand DTW-PA from 1.312 to 1.202, but R@1 drops from 70.25 to 16.36 and FID worsens from 0.060 to 0.217.
This confirms that DTW can reward temporally truncated predictions even when valid sign segments are removed and semantic retrieval quality collapses.

\begin{table}[t]
\centering
\caption{Length sensitivity of SOKE-style DTW on Phoenix-2014T.
All rows use the same generated motions from SRVQ full refinement.
Only the effective generated sequence length used during evaluation is truncated.}
\label{tab:supp_length_sensitivity}
\setlength{\tabcolsep}{3.6pt}
\resizebox{\columnwidth}{!}{%
\begin{tabular}{lccccc}
\toprule
Length scale & DTW-JPE-B$\downarrow$ & DTW-JPE-LH$\downarrow$ & DTW-PA-LH$\downarrow$ & FID$\downarrow$ & R@1$\uparrow$ \\
\midrule
1.0 & 5.299 & 6.877 & 1.312 & \textbf{0.060} & \textbf{70.25} \\
0.9 & 5.146 & 6.663 & 1.271 & 0.068 & 65.58 \\
0.8 & 5.031 & 6.522 & 1.241 & 0.089 & 53.12 \\
0.7 & 4.956 & 6.455 & 1.221 & 0.121 & 41.12 \\
0.6 & 4.896 & \textbf{6.390} & 1.208 & 0.162 & 28.50 \\
0.5 & \textbf{4.852} & 6.394 & \textbf{1.202} & 0.217 & 16.36 \\
\bottomrule
\end{tabular}}
\end{table}
